# Supplementary material for: Real or Not Real, that is the Question
Source: arXiv:2002.05512 source file (2020-02-12)
Supplement: Supplementary file 1 [file appendix.tex]

\newpage
\appendix

\section{Full proof on Theorem 1}
\begin{proof}                                                                              
Given a fixed $G$, the objective of $D$ is:
\begin{align}                                                                                            
\min_D V(G, D) & = \Ebb_{\vx \sim p_\text{data}}[\KL(\cA_1 \Vert D(\vx))] + \Ebb_{\vx \sim p_g}[\KL( \cA_0 \Vert D(\vx))], \\
      & = \int_\vx \left( p_\text{data}(\vx) \int_u \cA_1(u) \log \frac{\cA_1(u)}{D(\vx, u)}du + p_g(\vx) \int_u \cA_0(u) \log \frac{\cA_0(u)}{D(\vx, u)} du \right)dx, \\
	& = \int_\vx \left(p_\text{data}(\vx)h(\cA_1) + p_g(\vx) h(\cA_0)\right)dx \notag \\
	& - \int_\vx \int_u ( p_\text{data}(\vx) \cA_1(u) + p_g(\vx) \cA_0(u)) \log D(\vx, u) du dx, \label{eq:proof1_1}
\end{align}
where $h(\cA_1)$ and $h(\cA_0)$ are their entropies, and the first term in \eqref{eq:proof1_1} is irrelevant to $D$, marked as $C_1$.
The objective thus is equivalent to:
\begin{align}
	\min_D V(G, D) & = - \int_\vx \int_u (p_\text{data}(\vx) \cA_1(u) + p_g(\vx) \cA_0(u)) \log D(\vx, u) du dx + C_1, \\
	       & = - \int_\vx (p_\text{data}(\vx) + p_g(\vx)) \int_u \frac{p_\text{data}(\vx) \cA_1(u) + p_g(\vx)\cA_0(u)}{p_\text{data}(\vx) + p_g(\vx)}\log D(\vx, u) du dx + C_1,
\end{align}
where $p_\vx(u) = \frac{p_\text{data}(\vx) \cA_1(u) + p_g(\vx)\cA_0(u)}{p_\text{data}(\vx) + p_g(\vx)}$ is a distribution defined on $\Omega_u$.
Consequently, let $C_2 = p_\text{data}(\vx) + p_g(\vx)$, we have
\begin{align}
	\min_D V(G,D) & = C_1 + \int_\vx C_2 \left( - \int_u p_\vx(u) \log D(\vx, u) du + h(p_\vx) - h(p_\vx)\right) dx, \\
		& = C_1 + \int_\vx C_2 \KL( p_\vx \Vert D(\vx)) dx + \int_\vx C_2 h(p_\vx) dx. \label{eq:proof1_2}	
\end{align}
From \eqref{eq:proof1_2} we can see,
for any $\vx \in Supp(p_\text{data}) \cup Supp(p_g)$,
when $\KL( p_\vx \Vert D(\vx) )$ achieves its minimum,
$D$ obtains its optimal $D^\star$.
And at that time,
we have $D^\star(\vx) = p_\vx$,
which concludes the proof.
\end{proof}                                                                                                
